# Supplementary material for: DC-Prophet: Predicting Catastrophic Machine Failures in DataCenters
Source: arXiv:1709.06537 source file (2017-08-14)
Supplement: Supplementary file 1 [file 900appendix.tex]

\subsection*{Kolmogorov-Smirnov (K-S) test}
Kolmogorov-Smirnov test (K-S test) is a non-parametric statistical test for testing the equality of two probability distributions. The null hypothesis assumes the samples are drawn from the given continuous distribution. Mathematically, the Kolmogorov-Smirnov test statistic is defined as:
\begin{equation}
D_n = \sup_{x} |F_n(x) - F(x)|
\nonumber
\end{equation}
\noindent where $F_n(x)$ is the empirical distribution estimated from the sample population, and $F(x)$ is the cumulative distribution function (CDF) of the given probability distribution. Under the null hypothesis, $\sqrt{n} D_n$ converges to the Kolmogorov distribution. Hence, the risk region of Kolmogorov-Smirnov test is $\sqrt{n} D_n > K_{\alpha}$, where $K_{\alpha}$ satisfies that $P(K > K_{\alpha}) = 1-\alpha$, $K$ follows Kolmogorov distribution. 

%\subsection{Bayesian information criterion (BIC)}
%Bayesian information criterion(BIC) is a criterion for model selection. In model selection, the criterion
%purely based on log-likelihood is likely leading to over-fitting. BIC is a penalized version of log-likelihood.
%Mathematically, 
%\begin{equation}
%BIC = -2 L + k \ln(n)
%\nonumber
%\end{equation}
%\noindent where $L$ is log-likelihood, k is the number of parameters, and n is number of observations.
%Hence, minimizing BIC tends to select model with less parameters (parsimony). 

\subsection*{Kendall tau in Gumbel copula}
Kendall tau rank correlation $\Ken$ measures the dependency between two random variables. 
Given random variables $X$, $Y$ and $n$ pairs of their observations, $(x_1, y_1), \dots, (x_n, y_n)$, 
a pair of observations $(x_i, y_i)$ and $(x_j, y_j)$ is called concordant if $(x_i - x_j)(y_i - y_j) > 0$.
Likewise, the pair is called discordant if $(x_i - x_j)(y_i - y_j) < 0$. Hence, $\Ken$ is defined as:
\begin{equation}
\Ken = \frac{(\text{\# of concordant pairs}) - (\text{\# of discordant pairs})}{\frac{1}{2} n (n-1) }
\nonumber
\end{equation}
\noindent Note that $\Ken$ must be in $[-1,1]$. In particular, if $Y$ is rigorously increasing monotone with respect to $X$, $\Ken = 1$, whereas if $Y$ is rigorously decreasing monotone with respect to $X$, then $\Ken = -1$.
